# Supplementary material for: Learning the Truth From Only One Side of the Story
Source: arXiv:2006.04858 source file (2020-10-13)
Supplement: Supplementary file 1 [file plots_appendix_old.tex]

\newpage
\section{Additional Experiment Results}
\label{sec:appendix_simulation}
\qijia{I have slight preference for (1) not showing all range of $c$; (2) put table 3 below as an extra column in table 5.}

\begin{table}[H]
\begin{center}
\setlength{\tabcolsep}{8pt}
\begin{tabular}{|l|l|l|l|l|l|l|l|l|l|l|l|}
\hline
 c & 0.0 & 0.1 & 0.2 & 0.3 & 0.4 & 0.5 & 0.6 & 0.7 & 0.8 & 0.9 & 1.0\\  \hline
Adult & 78.6 & 62.0 & 50.5 & 36.4 & 23.9 & 15.9 & 10.0 & 6.6 & 4.4 & 3.0 & 1.7\\ \hline
Bank & 70.1 & 35.6 & 28.3 & 12.8 & 5.7 & 4.4 & 2.8 & 1.0 & 0.6 & 0.3 & 0.0\\ \hline
COMPAS & 100.0 & 98.3 & 86.2 & 72.1 & 55.5 & 39.8 & 27.1 & 16.0 & 7.7 & 2.0 & 0.2\\ \hline
Crime & 79.7 & 61.5 & 48.7 & 39.8 & 33.0 & 26.4 & 20.7 & 15.2 & 10.2 & 6.6 & 3.7
\\ \hline 
magic04 & 97.1 & 95.6 & 93.1 & 88.3 & 81.8 & 74.7 & 66.6 & 55.2 & 36.8 & 13.5 & 0.6\\ \hline
Banknote & 77.8 & 63.6 & 54.7 & 50.2 & 48.5 & 46.8 & 45.6 & 42.4 & 36.7 & 26.0 & 13.0 \\ 
\hline

\end{tabular}
\caption{\label{tab:linear_counts} {\bf Linear Regression Positive Examples}. For each dataset and each value of $c$, we show the percentage of dataset with linear model giving a prediction at least that $c$, where the linear model is trained on the entire dataset. }
\end{center}
\end{table}


\begin{table}[H]
\setlength{\tabcolsep}{8pt}
\begin{tabular}{|l|l|l|l|l|l|l|l|l|l|l|l|}
\hline
 & 0.0 & 0.1 & 0.2 & 0.3 & 0.4 & 0.5 & 0.6 & 0.7 & 0.8 & 0.9 & 1.0\\ \hline
Adult & 34.1 & 30.8 & 27.4 & 24.4 & 21.9 & 19.6 & 17.4 & 15.4 & 13.5 & 11.7 & 9.8\\ \hline
Bank & 13.8 & 11.6 & 9.9 & 8.4 & 7.0 & 5.8 & 4.9 & 4.4 & 3.9 & 3.5 & 2.9\\ \hline
COMPAS & 78.6 & 70.7 & 63.3 & 54.1 & 46.5 & 40.2 & 33.8 & 28.7 & 22.8 & 17.5 & 12.9\\ \hline
Crime & 37.3 & 34.8 & 32.5 & 30.8 & 29.4 & 27.3 & 25.5 & 24.0 & 22.6 & 20.6 & 18.8\\ \hline
magic04 & 86.3 & 83.5 & 80.9 & 78.2 & 75.5 & 72.9 & 69.8 & 66.5 & 62.9 & 58.1 & 52.3\\ \hline
Banknote & 43.6 & 42.9 & 41.5 & 41.0 & 40.7 & 40.3 & 39.8 & 39.2 & 38.3 & 37.6 & 37.0\\ \hline

\end{tabular}
\caption{\label{tab:logistic_counts} {\bf Logistic Regression Positive Examples}. For each dataset and each value of $c$, we show the percentage of dataset with logistic model giving a prediction at least that $c$, where the logistic model is trained on the entire dataset and the prediction is $\hat{y}_{1} - \hat{y}_{0} + 0.5$. }
\end{table}




\begin{table}[H]
\setlength{\tabcolsep}{8pt}
\centering
\begin{tabular}{|l|l|l|l|l|l|l|}
\hline
   & greedy & $\epsilon$-grdy & os-$\epsilon$-grdy   & noise           & os-noise        & ours        \\ \hline
Adult c=0   & 511.77 & 508.69     & 204.14          & 397.79          & 112.76          & \textbf{98.12}  \\ \hline
Adult c=0.1 & 406.64 & 402.1      & 267.07          & 365.73          & 198.23          & \textbf{152.66} \\ \hline
Adult c=0.2 & 263.14 & 251.89     & 223.84          & 240.54          & 170.34          & \textbf{146.01} \\ \hline
Adult c=0.3 & 129.68 & 129.06     & 128.75          & 127.64          & 123.37          & \textbf{115.72} \\ \hline
Adult c=0.4 & 155.92 & 155.32     & 155.14          & 155.81          & 161.25          & \textbf{152.98} \\ \hline
Adult c=0.5 & 222.79 & 221.85 & 223.23 & 220.88 & 220.12 & {\bf 219.42} \\ \hline
Adult c=0.6 & 320.5  & 299.58     & \textbf{296.98} & 299             & 306.34          & 301.51          \\ \hline
Adult c=0.7 & 230.67 & 218.14 & 209.27& 204.71 & 214.53 & {\bf 203.19}            \\ \hline
Adult c=0.8 & 144.89 & 137.05     & 140.91          & 133.36          & 126.9           & \textbf{124.17} \\ \hline
Adult c=0.9 & 136.14 & 135.05     & 129.83          & 116.51          & 115.78          & \textbf{97.01}  \\ \hline
Adult c=1   & 96.16  & 96.31      & 97.16           & 96.97           & 94.86           & \textbf{86.3}   \\ \hline
Bank c=0   & 297.9  & 294.08     & 124.71          & 216.69          & \textbf{71.32}  & 80.62           \\ \hline
Bank c=0.1 & 137.29 & 136.32     & 120.97          & 133.86          & 101.59          & \textbf{94}     \\ \hline
Bank c=0.2 & 214.59 & 213.2      & 205.64          & 209.87          & 177.72          & \textbf{155.44} \\ \hline
Bank c=0.3 & 113.08 & 112.61     & 112.09          & 111.51          & 116.67          & \textbf{111.08} \\ \hline
Bank c=0.4 & 115.35 & 113        & 113.27          & 114.35          & 117.32          & \textbf{112.2}  \\ \hline
Bank c=0.5 & 104.86 & 104.86 & {\bf 102.99} & 104.76 & 105.32 & 103.57      \\ \hline
Bank c=0.6 & 73.44  & 73         & 75.86           & \textbf{71.69}  & 76.44           & 73.41           \\ \hline
Bank c=0.7 & 53.14 & 52.65 & 53.47 & 51.39 & 50.4 & {\bf 47.91} \\ \hline
Bank c=0.8 & 34.64  & 34.57      & 35.47           & 34.01           & 36.97           & \textbf{33.64}  \\ \hline
Bank c=0.9 & 10.19  & 10.19      & 11.72           & 10.46           & 12.31           & \textbf{9.84}   \\ \hline
Bank c=1   & 3.71   & 3.81       & 5.35            & \textbf{3.61}   & 5.1             & 3.71            \\ \hline
COMPAS c=0   & 6.89   & 6.89       & \textbf{0}      & 7.39            & \textbf{0}      & 0.03            \\ \hline
COMPAS c=0.1 & 12.87  & 12.91      & \textbf{2.57}   & 12.32           & 2.91            & 2.94            \\ \hline
COMPAS c=0.2 & 26.21  & 25.72      & 15.2            & 24.03           & 12.72           & \textbf{11.2}   \\ \hline
COMPAS c=0.3 & 30.7   & 30.47      & 27.43           & 29.38           & 19.31           & \textbf{17.48}  \\ \hline
COMPAS c=0.4 & 35.42  & 34.96      & 32.94           & 34.46           & 28.99           & \textbf{25.2}   \\ \hline
COMPAS c=0.5 & 40.82  & 40.04      & 40.46           & 42.08           & \textbf{34.55}  & 36.6            \\ \hline
COMPAS c=0.6 & 43.15  & 40.28      & 37.53           & 38.78           & \textbf{34.53}  & 34.76           \\ \hline
COMPAS c=0.7 & 48.52  & 47.01      & 47.31           & 43.63           & 36.71           & \textbf{34.82}  \\ \hline
COMPAS c=0.8 & 34     & 33.74      & 33.97           & 33.09           & 34.66           & \textbf{32.8}   \\ \hline
COMPAS c=0.9 & 12.19  & 12.19      & 12.22           & 11.98           & 13.89           & \textbf{11.52}  \\ \hline
COMPAS c=1   & 5.39   & 5.51       & 5.63            & \textbf{4.92}   & 7.01            & 5.35            \\ \hline
Crime=0   & 21.7   & 21.64      & 16.26           & 22.02           & \textbf{11.98}  & 12.07           \\ \hline
Crime=0.1 & 17.43  & 17.41      & 17.38           & 17.14           & 15              & \textbf{14.08}  \\ \hline
Crime=0.2 & 15.55  & 15.55      & 15.4            & 15.97           & 15.04           & \textbf{14.27}  \\ \hline
Crime=0.3 & 18.2   & 18.12      & 18.16           & 18.4            & \textbf{16.83}  & 16.87           \\ \hline
Crime=0.4 & 21.56  & 21.48      & 21.66           & 22.29           & 20.75           & \textbf{20.22}  \\ \hline
Crime=0.5 & 20.88  & 20.88      & 21              & 20.95           & 22.27           & \textbf{20.67}  \\ \hline
Crime=0.6 & 27.96  & 27.51      & 28.21           & 26.13           & \textbf{23.61}  & 24.38           \\ \hline
Crime=0.7 & 19.89  & 19.89      & 19.96           & 21.52           & 20.91           & \textbf{19.82}  \\ \hline
Crime=0.8 & 22.59  & 22.59      & 22.68           & 21.38           & \textbf{20.56}  & 21.19           \\ \hline
Crime=0.9 & 15.2   & 15.2       & 15.63           & 15.47           & 16.54           & \textbf{14.86}  \\ \hline
Crime=1   & 10.11  & 10.11      & 10.19           & 10.14           & 11.52           & \textbf{10}     \\ \hline
   magic04  c=0   & 61.926 & 62.052 & 35.784          & 60.783         & 18.716          & \textbf{11.938} \\ \hline
magic04  c=0.1 & 52.131 & 52.068 & 38.68           & 51.958         & 21.831          & \textbf{16.288} \\ \hline
magic04  c=0.2 & 50.52  & 50.27  & 41.217          & 49.467         & 26.906          & \textbf{19.862} \\ \hline
magic04  c=0.3 & 66.42  & 66.42  & 53.997          & 63.397         & 28.862          & \textbf{25.176} \\ \hline
magic04  c=0.4 & 79.421 & 78.383 & 68.465          & 75.834         & 33.911          & \textbf{31.026} \\ \hline
magic04  c=0.5 & 81.73  & 81.614 & 76.869          & 79.979         & 39.963          & \textbf{38.404} \\ \hline
magic04  c=0.6 & 78.452 & 77.344 & 75.482          & 77.004         & \textbf{50.019} & 52.547          \\ \hline
magic04  c=0.7 & 113.57 & 113    & 112.67          & 113.03         & \textbf{85.216} & 87.483          \\ \hline
magic04  c=0.8 & 216.03 & 216.03 & 214.37          & 213.38         & \textbf{202.04} & 210.29          \\ \hline
magic04  c=0.9 & 267.29 & 263.95 & \textbf{261.14} & 258.28         & 264.18          & 266.1           \\ \hline
magic04  c=1   & 14.709 & 14.714 & 15.239          & \textbf{13.18} & 14.556          & 14.717          \\ \hline
\end{tabular}
\caption{\label{tab:linear_table_all}  { Linear Regression Results}. }
\end{table}



\begin{table}[H]
\centering
\begin{tabular}{|l|l|l|l|l|l|l|}
\hline
   & greedy & $\epsilon$-grdy & os-$\epsilon$-grdy   & noise           & os-noise        & ours        \\ \hline
Adult c=0       & 274.54          & 274.11              & 274.62                 & 273.96          & 273.16            & \textbf{266.77}   \\ \hline
Adult c=0.1       & 269.16          & 269.07              & 268.46                 & 267.87          & 266.36            & \textbf{263.84}   \\ \hline
Adult c=0.2       & 256.08          & 256.15              & 256.18                 & 255.19          & 253.67            & \textbf{251.72}   \\ \hline
Adult c=0.3       & 222.64          & 222.25              & 222.42                 & 221.84          & 220.77            & \textbf{216.91}   \\ \hline
Adult c=0.4       & 219.85          & 219.84              & 220.2                  & 219.31          & 217.99            & \textbf{215.11}   \\ \hline
Adult c=0.5          & 205.19 & 205.44 & 205.76 & 203.27 & 203.49 & {\bf 196.3}  \\ \hline
Adult c=0.6        & 167.93          & 168.08              & 168.19                 & 167.45          & 166.64            & \textbf{165.43}   \\ \hline
Adult c=0.7        &  173.26 & 173.43 & 173.26 & 172.39 & 172.79 & {\bf 171.08}      \\ \hline
Adult c=0.8        & 145             & 145.09              & 145.13                 & 143.59          & 144.73            & \textbf{144.29}   \\ \hline
Adult c=0.9        & 136.17          & 136.17              & 136.31                 & 135.75          & \textbf{135.24}   & 135.5             \\ \hline
Adult c=1        & 116.11          & 116.36              & 116.41                 & \textbf{113.82} & 114.01            & 114.3             \\ \hline
Bank c=0       & 165.52          & 164.3               & 165.27                 & 164.81          & \textbf{162.92}   & 163.54            \\ \hline
Bank c=0.1       & 155.95          & 155.33              & 155.55                 & 153.79          & 153.01            & \textbf{147.49}   \\ \hline
Bank c=0.2       & 146.96          & 146.16              & 146.82                 & 145.48          & 144.8             & \textbf{139.54}   \\ \hline
Bank c=0.3       & 144.25          & 143.96              & 144.71                 & 142.05          & 140.42            & \textbf{130.91}   \\ \hline
Bank c=0.4       & 134.14          & 134.14              & 134.28                 & 131.1           & 132.49            & \textbf{127.44}   \\ \hline
Bank c=0.5         & 129.04          & 128.67              & 129.3                  & 128.51          & 127.07            & \textbf{124.26}   \\ \hline
Bank c=0.6        & 117.79          & 117.9               & 118.77                 & 116.75          & 117.87            & \textbf{108.05}   \\ \hline
Bank c=0.7        & 123.44          & 123.55              & 124.34                 & 122.82          & 121.01            & \textbf{105.11}   \\ \hline
Bank c=0.8        & 117.05          & 117.27              & 117.27                 & 115.08          & 115.97            & \textbf{95.58}    \\ \hline
Bank c=0.9        & 97.36           & 97.36               & 97.68                  & 96.9            & 95.93             & \textbf{83.32}    \\ \hline
Bank c=1        & 78.96           & 78.87               & 79.61                  & 78.65           & 77.81             & \textbf{70.94}    \\ \hline
COMPAS c=0       & 25.3 & 25.3 & 25.02 & 24.94 & 20.03 & {\bf 17.54}  \\ \hline
COMPAS c=0.1       & 30.38 & 30.34 & 29.84 & 29.27 & 27.07 & {\bf 23.51}    \\ \hline
COMPAS c=0.2       & 39.2 & 39.07 & 39.2 & 39.12 & 34.01 & {\bf 28.7}   \\ \hline
COMPAS c=0.3       & 32.63 & 32.49 & 32.57 & 31.67 & 31.5 & {\bf 29.87}   \\ \hline
COMPAS c=0.4       &  38.08 & 38.02 & 38.0 & 37.0 & {\bf 36.37} & 37.44  \\ \hline
COMPAS c=0.5    &    43.53 & 43.5 & 43.53 & 43.13 & 42.78 & {\bf 42.46}     \\ \hline
COMPAS c=0.6        & 33.7 & 33.64 & 33.7 & 33.21 & 33.42 &  {\bf 33.05}      \\ \hline
COMPAS c=0.7        & 32.5 & 32.5 & 32.58 & 32.41 & 31.94 & {\bf 31.56}    \\ \hline
COMPAS c=0.8        & 34.14 & 34.14 & 34.14 & 33.84 & 33.16 & {\bf 32.62}    \\ \hline
COMPAS c=0.9        & 31.01 & 31.01 & 30.87 & 30.89 & 31.05 & {\bf 30.61}        \\ \hline
COMPAS c=1        &30.21 & 29.57 & 29.77 & 28.98 & {\bf 27.8} & 29.07  \\ \hline
Crime c=0    & 20.97 & 20.97 & 20.99 & 20.14 & 20.18 & {\bf 19.95}   \\ \hline
Crime c=0.1       & 20.58 & 20.58 & 20.58 & 20.64 & 20.03 & {\bf 18.61}   \\ \hline
Crime c=0.2      & 21.96 & 21.96 & 21.98 & 21.97 & 21.43 & {\bf 20.04}   \\ \hline
Crime c=0.3       & 27.56 & 27.56 & 27.64 & 26.52 & 24.79 & {\bf  24.45}            \\ \hline
Crime c=0.4      & 26.57 & 26.57 & 26.57 & 26.4 & {\bf 25.58} & 25.62            \\ \hline
Crime c=0.5          & 25.75 & 25.75 & 25.75 & 26.14 & 25.46 & {\bf 24.58}        \\ \hline
Crime c=0.6       & 28.55 & 28.55 & 28.55 & 27.4 & 27.53 & {\bf 27.31}          \\ \hline
Crime c=0.7        & 26.49 & 26.49 & 26.55 & 25.85 & 25.95 & {\bf 25.57}           \\ \hline
Crime c=0.8    &   26.18 & 26.3 & 26.18 & 26.18 & {\bf 26.11} & 26.18         \\ \hline
Crime c=0.9        &  25.46 & 25.46 & 25.3 & {\bf 24.79} & 24.91 & 25.08        \\ \hline
Crime c=1        &  24.74 & 24.74 & 24.68 & 24.26 & {\bf 24.08} & 24.47         \\ \hline
magic04  c=0 & 128.1           & 122.1           & 121.61          & 121.9           & 90.381          & \textbf{88.677} \\ \hline
magic04  c=0.1 & 182.08          & 176.31          & 177.38          & 175.51          & \textbf{118.64} & 125.2           \\ \hline
magic04  c=0.2 & 196.53          & 193.08          & 191.09          & 189.29          & \textbf{147.63} & 147.8           \\ \hline
magic04  c=0.3 & 202.51          & 203.91          & 204.22          & 204.16          & 172.18          & \textbf{157.59} \\ \hline
magic04  c=0.4 & 244.17          & 237.22          & 235.77          & 234.53          & 191.26          & \textbf{179.51} \\ \hline
magic04  c=0.5    & 263.68          & 263.32          & 263.19          & 263.8           & 220.86          & \textbf{206.64} \\ \hline
magic04  c=0.6  & 258.63          & 258.34          & 258.41          & 255.94          & 232.59          & \textbf{218.39} \\ \hline
magic04  c=0.7  & 245.06          & 242.43          & 242.86          & 241.32          & 226.97          & \textbf{225.35} \\ \hline
magic04  c=0.8  & 257.2           & 254.76          & 256.66          & 255.91          & 245.06          & \textbf{237.44} \\ \hline
magic04  c=0.9  & 271.51          & 266.39          & 267.52          & 266.66          & \textbf{263.03} & 264.66          \\ \hline
magic04  c=1  & 273.52          & 274.1           & 275.07          & \textbf{270.11} & 273.3           & 271.7           \\ \hline
\end{tabular}
\caption{\label{tab:logistic_table_all} { Logistic Regression Results}.}
\end{table}


 \begin{figure}[H]
  \begin{center}
    \includegraphics[width=0.45\textwidth]{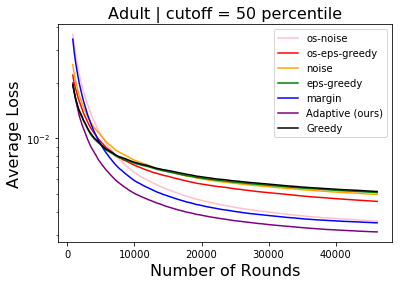}
    \includegraphics[width=0.45\textwidth]{figures/linear_adult_all_0_7.png}
    \includegraphics[width=0.4\textwidth]{figures/linear_bank_all_0_5.png}
    \includegraphics[width=0.45\textwidth]{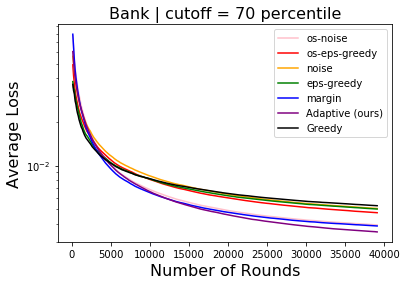}
    \includegraphics[width=0.45\textwidth]{figures/linear_compas_all_0_5.png}
    \includegraphics[width=0.45\textwidth]{figures/linear_compas_all_0_7.png}
    \includegraphics[width=0.45\textwidth]{figures/linear_crime_all_0_5.png}
    \includegraphics[width=0.45\textwidth]{figures/linear_crime_all_0_7.png}
    \includegraphics[width=0.45\textwidth]{figures/linear_magic04_all_0_5.png}
    \includegraphics[width=0.45\textwidth]{figures/linear_magic04_all_0_7.png}
    \end{center}
  \caption{{ Linear Regression plots for all datasets}. }
	\label{fig:linear_plots_all}
\end{figure}



 \begin{figure}[H]
  \begin{center}
    \includegraphics[width=0.45\textwidth]{figures/logistic_adult_all_0_5.png}
    \includegraphics[width=0.45\textwidth]{figures/logistic_adult_all_0_7.png}
    \includegraphics[width=0.45\textwidth]{figures/logistic_bank_all_0_5.png}
    \includegraphics[width=0.45\textwidth]{figures/logistic_bank_all_0_7.png}
    \includegraphics[width=0.45\textwidth]{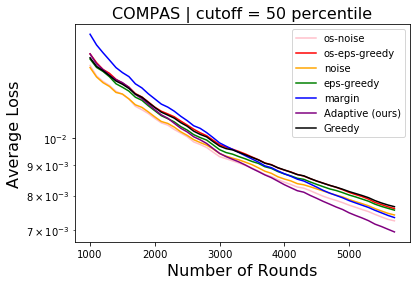}
    \includegraphics[width=0.45\textwidth]{figures/logistic_compas_all_0_7.png}
    \includegraphics[width=0.45\textwidth]{figures/logistic_crime_all_0_5.png}
    \includegraphics[width=0.45\textwidth]{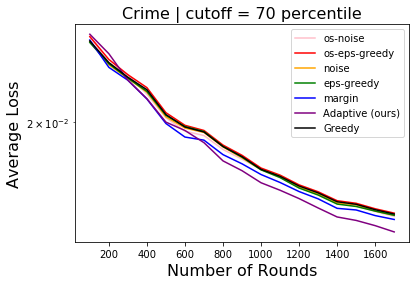}
    \includegraphics[width=0.45\textwidth]{figures/logistic_magic04_all_0_5.png}
    \includegraphics[width=0.45\textwidth]{figures/logistic_magic04_all_0_7.png}
    \end{center}
  \caption{{ Logistic Regression plots for all datasets}. }
	\label{fig:logistic_plots__all}
\end{figure}
